# Supplementary material for: KIF: Knowledge Identification and Fusion for Language Model Continual Learning
Source: arXiv:2408.05200 source file (2025-01-23)
Supplement: Supplementary file 1 [file 8.appendix.tex]

Table \ref{superni} \& \ref{long-sequence} show details of the datasets we used for our experiments, along with their evaluation metrics. Overall, in SuperNI, we choose 3 tasks from dialogue generation (Dialog), information extraction (IE),  question answering (QA), summarization (Sum) and sentiment analysis (SA), respectively.

For the Long Sequence benchmark, this includes five tasks from the standard CL benchmark (AG News, Amazon reviews, Yelp reviews, DBpedia and Yahoo Answers), four from GLUE benchmark (MNLI, QQP, RTE, SST2), five from SuperGLUE benchmark (WiC, CB, COPA, MultiRC, BoolQ), and the IMDB movie reviews dataset.
%\subsection{Task Sequence Orders}
We report 4 different task orders used for our experiments in Table \ref{order}.

\begin{table*}
\caption{The details of 15 datasets in the SuperNI Benchmark \cite{wang2022super}.
}
\centering
\begin{tabular}{lllll}
\toprule
\textbf{Dataset name} & \textbf{Task}  & \textbf{Metric} \\
\midrule
1. task639\_multi\_woz\_user\_utterance\_generation  & dialogue generation   & Rouge-L        \\
2. task1590\_diplomacy\_text\_generation & dialogue generation   & Rouge-L       \\
3. task1729\_personachat\_generate\_next & dialogue generation   & Rouge-L      \\
4. task181\_outcome\_extraction & information extraction & Rouge-L        \\
5. task748\_glucose\_reverse\_cause\_event\_detection & information extraction & Rouge-L       \\
6. task1510\_evalution\_relation\_extraction   & information extraction & Rouge-L  \\
7. task002\_quoref\_answer\_generation & question answering & Rouge-L \\
8. task073\_commonsenseqa\_answer\_generation & question answering & Rouge-L    \\
9. task591\_sciq\_answer\_generation  & question answering & Rouge-L        \\
10. task511\_reddit\_tifu\_long\_text\_summarization     & summarization        & Rouge-L        \\
11. task1290\_xsum\_summarization  & summarization       & Rouge-L        \\
12. task1572\_samsum\_summary  &summarization  & Rouge-L \\
13. task363\_sst2\_polarity\_classification  & sentiment analysis   & accuracy        \\
14. task875\_emotion\_classification & sentiment analysis   & accuracy  \\
15. task1687\_sentiment140\_classification & sentiment analysis   & accuracy  \\
\bottomrule
\end{tabular}
\label{superni}
\end{table*}

\begin{table*}[htbp]
\caption{The details of 15 classification datasets in the Long Sequence Benchmark \cite{razdaibiedina2022progressive}. First five tasks
correspond to the standard CL benchmark \cite{zhang2015character}.
}
\centering
\begin{tabular}{lllll}
\toprule
\textbf{Dataset name} & \textbf{Category} & \textbf{Task}             & \textbf{Domain}     & \textbf{Metric} \\ \midrule
1. Yelp               & CL Benchmark      & sentiment analysis        & Yelp reviews        & accuracy        \\
2. Amazon             & CL Benchmark      & sentiment analysis        & Amazon reviews      & accuracy        \\
3. DBpedia            & CL Benchmark      & topic classification      & Wikipedia           & accuracy        \\
4. Yahoo              & CL Benchmark      & topic classification      & Yahoo Q\&A          & accuracy        \\
5. AG News            & CL Benchmark      & topic classification      & news                & accuracy        \\
6. MNLI               & GLUE              & natural language
inference                       & various             & accuracy        \\
7. QQP                & GLUE              & paragraph detection       & Quora               & accuracy        \\
8. RTE                & GLUE              & natural language inference                       & news, Wikipedia     & accuracy        \\
9. SST-2              & GLUE              & sentiment analysis        & movie reviews       & accuracy        \\
10. WiC               & SuperGLUE         & word sense disambiguation & lexical databases   & accuracy        \\
11. CB                & SuperGLUE         & natural language
inference                       & various             & accuracy        \\
12. COPA              & SuperGLUE         & question and answering                        & blogs, encyclopedia & accuracy        \\
13. BoolQA            & SuperGLUE         & boolean question and answering                & Wikipedia           & accuracy        \\
14. MultiRC           & SuperGLUE         & question and answering                        & various             & accuracy        \\
15. IMDB              & SuperGLUE         & sentiment analysis        & movie reviews       & accuracy        \\ \bottomrule
\end{tabular}
\label{long-sequence}
\end{table*}

\begin{table*}
\caption{Four different orders of task sequences used for our experiments. Orders
1-2 correspond to the SuperNI benchmark. Orders 3-4 are long-sequence orders following \cite{razdaibiedina2022progressive}.}
\centering
\begin{tabular}{lll}
\toprule
\textbf{Order} & \textbf{Model} & \textbf{Task Sequence}                                                                                                                                \\ 
\midrule
1              & T5, LLaMA-2      & \begin{tabular}[c]{@{}l@{}}task1572 → task363 → task1290 → task181 → task002 →\\ task1510 → task639 → task1729 → task073 → task1590 →\\ task748 → task511 → task591 → task1687 → task875\end{tabular} \\
2              & T5, LLaMA-2     & \begin{tabular}[c]{@{}l@{}}task748 → task073 → task1590 → task639 → task1572 →\\ task1687 → task591 → task363 → task1510 → task1729 →\\ task181 → task511 → task002 → task1290 → task875\end{tabular} \\
\midrule
3              & T5, LLaMA-2             & \begin{tabular}[c]{@{}l@{}}mnli → cb → wic → copa → qqp → boolqa → rte → imdb →\\ yelp → amazon → sst-2 → dbpedia → ag → multirc → yahoo\end{tabular} \\
4              & T5, LLaMA-2             & \begin{tabular}[c]{@{}l@{}}yelp → amazon → mnli → cb → copa → qqp → rte → imdb →\\ sst-2 → dbpedia → ag → yahoo → multirc → boolqa → wic\end{tabular} \\
\bottomrule
\end{tabular}
\label{order}
\end{table*}

% \begin{figure*}[t]
%   \centering
%   \includegraphics[width=1\linewidth]{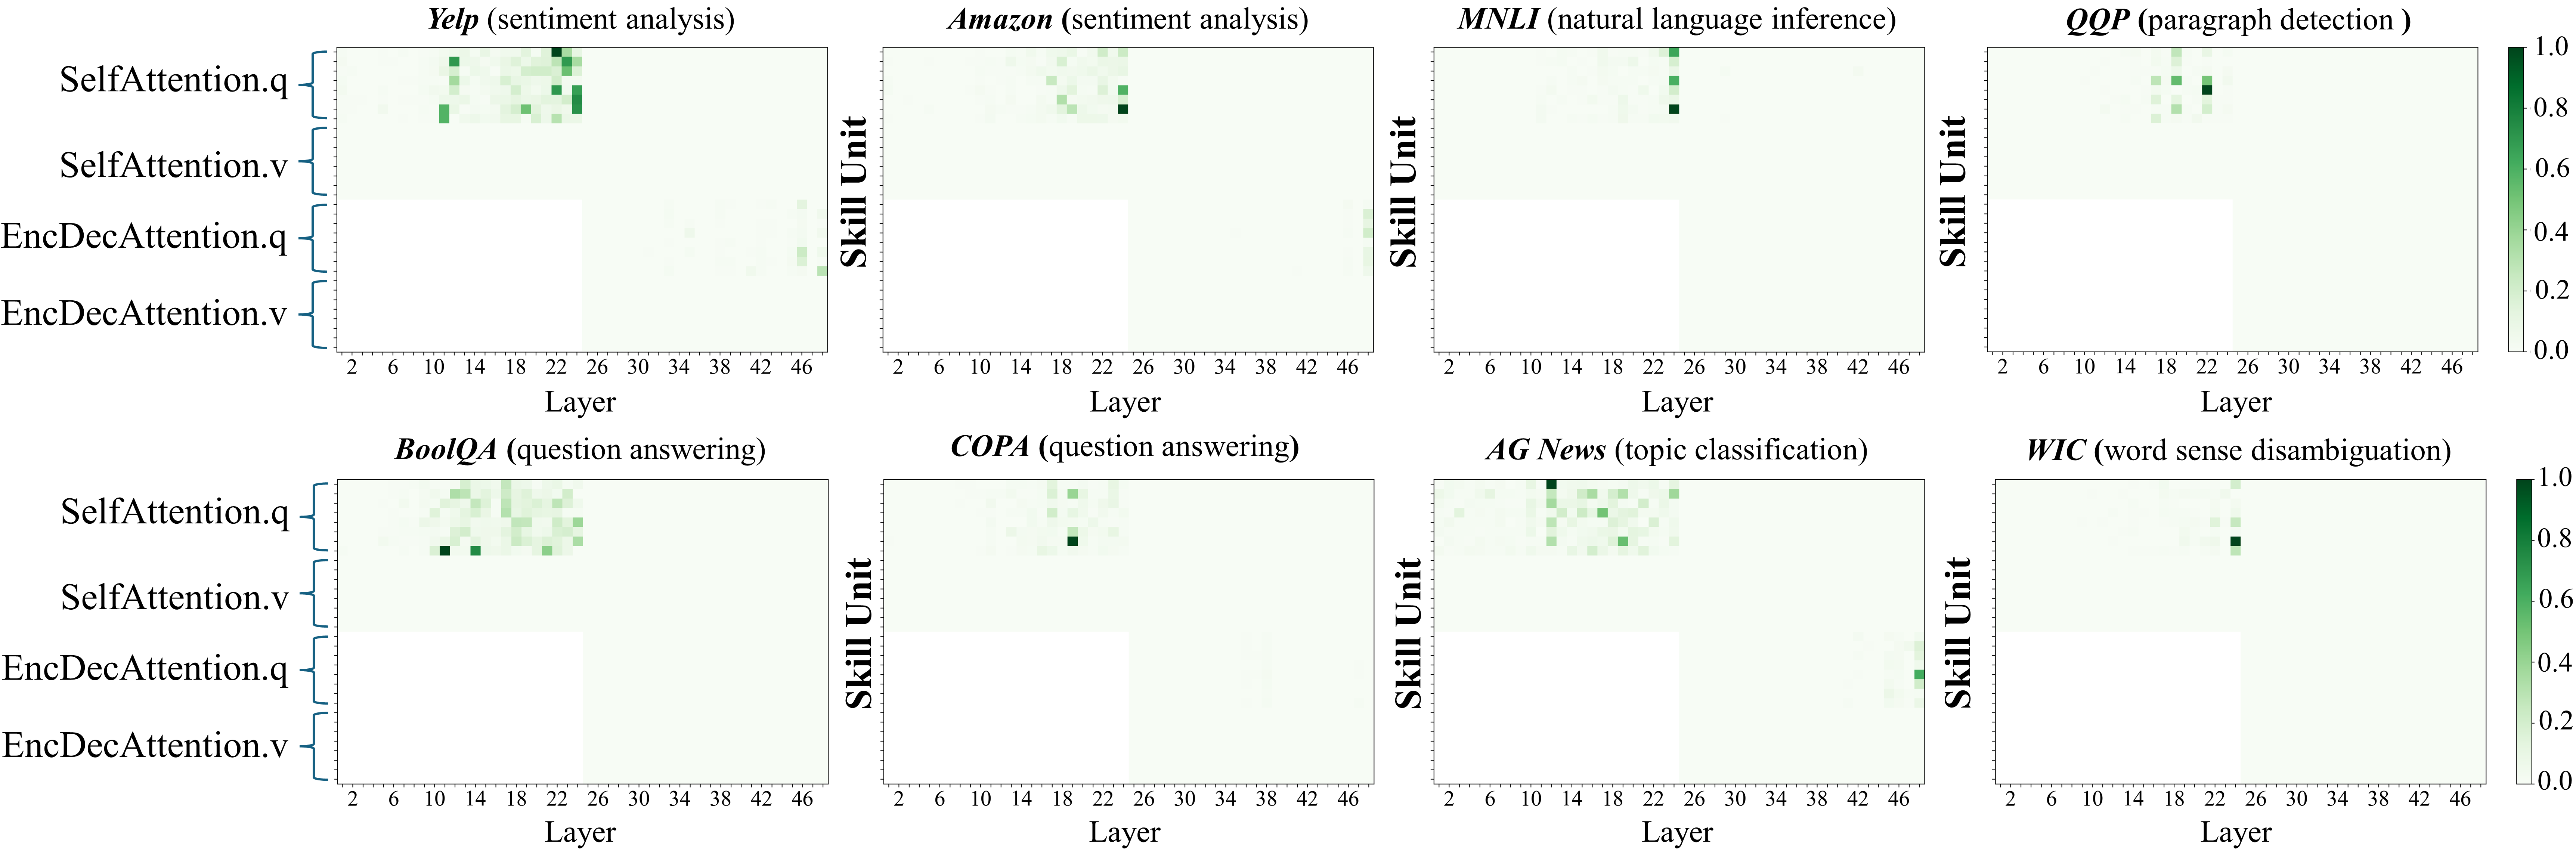}
%   \caption{Visualization of importance distributions for skill units across 15 different tasks on T5-large for the Long Sequence Benchmark. It reveals that for classification tasks, the parameters in the lower layers, particularly the Query matrix in the attention mechanism, play a more important role.}
%   \label{fig:heatmap_long}
% \end{figure*}

% \begin{figure*}[t]
%   \centering
%   \includegraphics[width=1\linewidth]{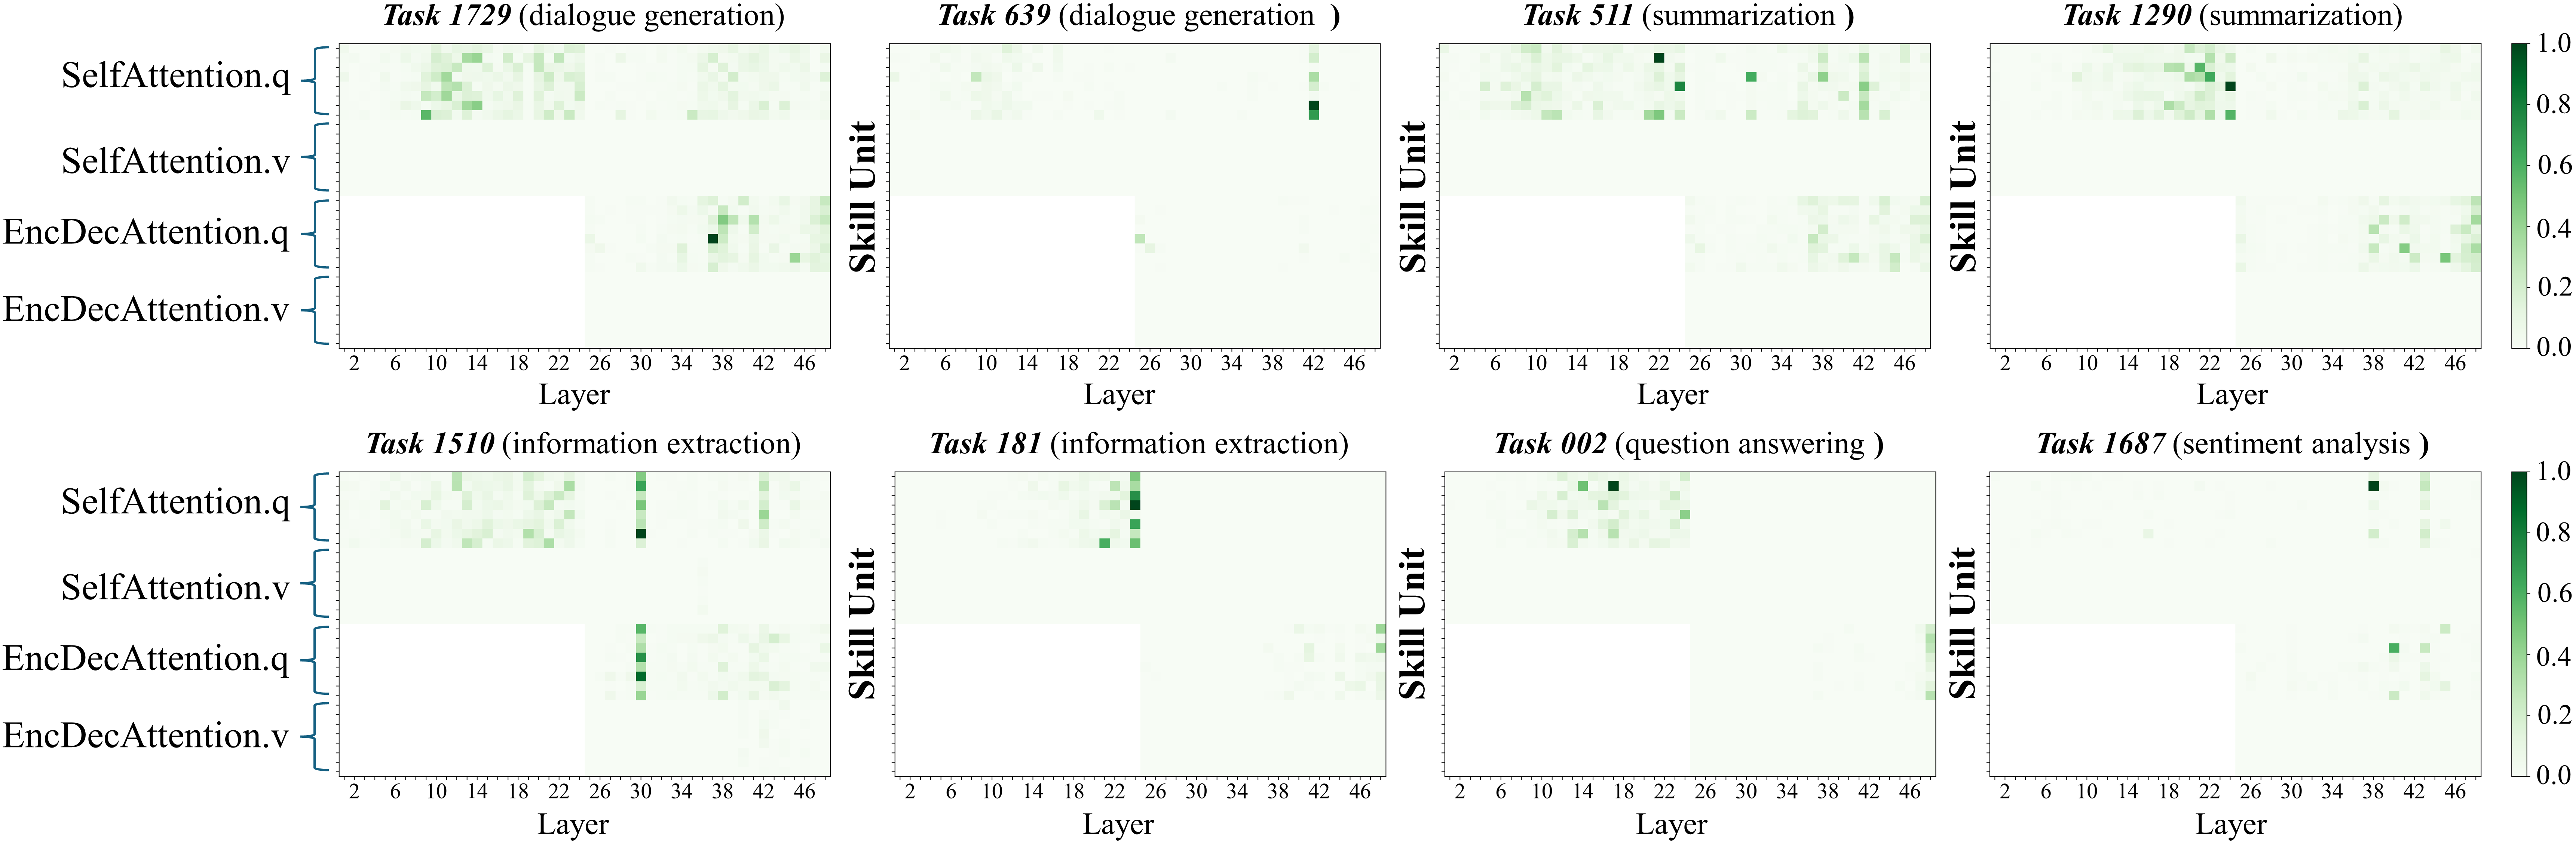}
%   \caption{Visualization of importance distributions for skill units across 15 different tasks on T5-large for the SuperNI Benchmark. It reveals that for generation tasks, both the parameters in the lower and upper layers of the network are important.
%   }
%   \label{fig:heatmap_superni}
% \end{figure*}
